# Supplementary material for: Understanding and Mitigating the Effect of Outliers in Fair Ranking
Source: arXiv:2112.11251 source file (2022-01-03)
Supplement: Supplementary file 1 [file 09-appendix.tex]

% !TEX root = ../main.tex
\newpage
\section*{Appendix}
\label{section:appendix}
\subsection*{Degrees of Outlierness}
%TODO change format of appendix to full page or adjust examples to work with this format. 

\if0
Outliers are exceptional items that deviate from the rest of the data\citep{wen-2006-ranking}. The problem of outlier detection is a fundamental issue in data mining, specifically in fraud detection, network intrusion, medical problems, network monitoring, etc. 

%Various outlier detection methods have been proposed in the last few decades, including linear models like Minimum Covariance Determinant (MCD)\cite{}, and One-class Support Vector Machines\cite{} [Move this to related work]

%To measure the outlierness of items in a list we need to find a way to determine whether an item should be marked as an outlier. There are two aspects to this problem: the first one is the feature(s) that are important to us to define an outlier, and the second one is the outlier detection method. In this section we propose four different approaches for this task and later on in the experiments we compare the results achieved from using each of them. 

Most outlier detection methods are designed to deal with big datasets, however since in our case the number of items retrieved as response to a query are limited, we choose heuristics that work fine for small datasets. On the other hand, the detection method should be able to handle big dimensionality of the data in case we want to use a large number of features to detect the outlierness of an item. To this end we also employ a recently introduced method, COPOD\cite{li2020copod}, which is a deterministic and efficient model and an ideal choice for high dimensionality data.

To this end, we use Interquartile Range (IQR) to measure the statistical dispersion and data variability by dividing the scores into quartiles. In general, using IQR, any dataset or any set of observations is divided into four defined intervals based upon the values of the data and how they compare to the entire dataset. A quartile is what divides the data into three points and four intervals.

IQR is used to define the outliers. IQR is the difference between the third quartile and the first quartile $IQR = Q3 -Q1$. Outliers are defined as the observations that are below $Q1 - 1.5 \times IQR$ or above $Q3 + 1.5 \times IQR$.

Using IQR we can calculate the degree of outlierness (if any) of the items in the top-k positions of the ranked list. By minimizing this value we can make sure that we are showing items in a way that the exposure is only dependant on the position of the item and not influenced by the effects of an outlier.

\fi

\subsection{Generalization of the BvN decomposition for potentially symmetric matrices}
%TODO maybe rename to pre-symmetric matrices. Search more for literature 

\subsubsection{Motivation}

The constructive proof of the Birkhoff-von Neumann theorem gives us a method to decompose any doubly stochastic matrix into the convex sum of permutation matrices. This can be used to derive an executable policy from a the Marginal Rank Probability matrix (MRP), which encodes a probabilistic (but not executable) policy that re-ranks the items in the list under certain fairness constraints. The theorem however does not provide us with an approach for deriving a decomposition in the top-$k$ setting. In this case the MRP will be non-squared and hence also not doubly stochastic. Nevertheless we can use the properties of such a matrix to derive a decomposition into a convex sum of permutation matrices from the BvN theorem. 

\subsubsection{BvN decomposition for potentially doubly stochastic matrices.}

For a doubly stochastic matrix $A$ the theorem by Birkhoff and von Neumann  %need citation, make sure theorem is from both
proves that $A$ can be decomposed into a convex sum of permutation matrices $A = \sum_i \alpha_i \cdot P_i$. The constructive proof of this theorem gives us a method to find such a decomposition. We want to adjust this method for the following class of matrices: We call a matrix $A=\{a_{i,j}\}_{i<k,j<n}$ potentially doubly stochastic % check whether those matrices are defined somewhere. 
if $\forall i,j: 0 \le a_{i,j} \le 1$ and for either  $A$ or $A^\top$: $\forall j \sum_{i} a_{i,j} = 1$ and   $\forall i \sum_{j} a_{i,j} \le 1$.  

We will show that such potentially doubly stochastic matrices can be filled up to doubly stochastic matrices. We will then use this fact to prove that each potentially doubly stochastic matrix can be decomposed into a linear combination of %partial? 
permutation matrices. 

\begin{lemma}
Let $A=\{a_{i,j}\}_{i<k,j<n}$ be a potentially doubly stochastic matrix with $k<n$. Then there is a matrix $A'=\{a'_{i,j}\}_{i,j<n}$ with $\forall i,j: 0 \le a'_{i,j} \le 1$ such that $A = \{a'_{i,j}\}_{i<k,j<n}$,  and $\forall i \sum_{i} a'_{i,j} = 1$ and $\forall j \sum_{i} a'_{i,j} = 1$. 
\end{lemma}
\begin{proof}
Define $A' = \{a'_{i,j}\}_{i,j<n}$ as 
\[
a'_{i,j} = \left\{
\begin{array}{ll}
a_{i,j} & j \le k \\
\frac{1 - \sum_{j'=1}^{} a_{i,j'}}{n - k}  & j > k \\
\end{array}
\right. 
\]
By definition we have $A = \{a'_{i,j}\}_{i<k,j<n}$. Furthermore, since $0 \le \sum_{j} a_{i,j} \le 1$ we also have $0 \le \frac{1 - \sum_{j'=1}^{} a_{i,j'}}{n - k} \le 1$. Furthermore for all $i < n $
\begin{align*}
    \sum_{j=1}^n a'_{i,j} & = \sum_{j=1}^k a_{i,j} + \sum_{j=k+1}^n \frac{1 - \sum_{j'=1}^{} a_{i,j'}}{n - k} \\
    &= \sum_{j=1}^k a_{i,j} + (n-k) \cdot  \frac{1 - \sum_{j'=1}^{k} a_{i,j'}}{n - k} \\
    &= \sum_{j=1}^k a_{i,j} + (1 - \sum_{j'=1}^{k} a_{i,j'})\\
    &= 1
\end{align*}
where we used in the second equality that we sum over $(n-k)$ times the same value. We know that the columns of the matrix sum to 1 for all $j\le k$, since this is the case for matrix $A$. For $j>k$ we have: 
\begin{align*}
    \sum_{i=1}^n a'_{i,j} & = \frac{1}{n-k} (\sum_{j=k}^n\sum_{i=1}^n a'_{i,j})\\
    & = \frac{1}{n-k}(n-\sum_{j=1}^k\sum_{i=1}^n a'_{i,j})\\ 
    & = \frac{n-k}{n-k} = 1 
\end{align*}
Here in the first equality we used that all columns from the $k$-th column are the same. In the second equality we used that since all rows are summing to $1$, the sum of all rows (and therefore also the sum of all columns) equals $n$. The last equality simply uses the fact that each of the first $k$ columns sums to $1$. 
\end{proof}
Note that by transposing $A$ we can show that the Lemma also holds in the case that $k>n$. 

This lemma leads us directly to the theorem on the existence of a decomposition for a potentially doubly stochastic matrix $A$ into a convex sum of permutation matrices. 
\begin{theorem}
We can write any potentially doubly stochastic matrix $A$ as the convex sum $A=\sum_{l=1}^m \alpha_l \cdot P_l$ of permutation matrices $P_l$ and coefficients $\alpha_l \in [0,1]$ with $\sum_{i=1}^m \alpha=1$.  
\end{theorem}
\begin{proof}
Without loss of generality let $k\le n$ In Lemma 1 we give a constructive proof that $A$ can be extended to a doubly stochastic matrix $A'$. For such a matrix the theorem by Birkhoff and Neumann % TODO cite 
states that we can find a decomposition $A' = \sum_{l=1}^m \alpha_l P'_l$ with $\alpha_l \in [0,1]$, $\sum_{i=1}^m \alpha=1$ and $P'_l= \{p^l_{i,j}\}_{i,j<n}$. Let $P_l=\{p^l_{i,j}\}_{i<n,j<k}$ be the matrix containing the first $k$ columns of $P_l$. Then $A = \sum_{l=1}^m \alpha_l P_l$. 
\end{proof}

While extending the matrix to a doubly stochastic matrix and using the Birkhoff von Neumann decomposition algorithm will certainly provide us with a decomposition, this is not the most efficient way to find a decomposition. Consider the following example:
\begin{equation*}
A = 
\begin{pmatrix}
0.2 & 0 \\
0 & 0.2  \\
0.8 & 0  \\
0 & 0.8 \\
\end{pmatrix}
A' = 
\begin{pmatrix}
0.2 & 0  &  \aug & 0.4& 0.4\\
0 & 0.2  &  \aug & 0.4& 0.4\\
0.8 & 0  &  \aug & 0.1& 0.1\\
0 & 0.8  &  \aug & 0.1& 0.1\\
\end{pmatrix}
\end{equation*} 
We can see that a decomposition of $A$ can be given by 
\begin{equation*}
A = 
\begin{pmatrix}
0.2 & 0 \\
0 & 0.2  \\
0.8 & 0  \\
0 & 0.8 \\
\end{pmatrix} = 
0.2 \cdot 
\begin{pmatrix}
0.1 & 0 \\
0 & 0.1  \\
0 & 0  \\
0 & 0 \\
\end{pmatrix} +
0.8 \cdot
\begin{pmatrix}
0 & 0 \\
0 & 0  \\
0.1 & 0  \\
0 & 0.1 \\
\end{pmatrix} 
\end{equation*} 
Nevertheless if we extend $A$ to $A'$ as we did in the Lemma the algorithm will have a longer runtime and use 4 instead of 2 matrices. This is due to the fact that we distribute the remaining row-sum value over the columns we need to fill up:  
\begin{align*}
A' = 
\begin{pmatrix}
0.2 & 0  &  \aug & 0.4& 0.4\\
0 & 0.2  &  \aug & 0.4& 0.4\\
0.8 & 0  &  \aug & 0.1& 0.1\\
0 & 0.8  &  \aug & 0.1& 0.1\\
\end{pmatrix}
&= 
0.1 \cdot 
\begin{pmatrix}
1 & 0  &  \aug & 0& 0\\
0 & 1  &  \aug & 0& 0\\
0 & 0  &  \aug & 1& 0\\
0 & 0  &  \aug & 0& 1\\
\end{pmatrix}
+ 0.1 \cdot 
\begin{pmatrix}
1 & 0  &  \aug & 0& 0\\
0 & 1  &  \aug & 0& 0\\
0 & 0  &  \aug & 0& 1\\
0 & 0  &  \aug & 1& 0\\
\end{pmatrix}\\ 
&+ 0.4 \cdot 
\begin{pmatrix}
0 & 0  &  \aug & 1& 0\\
0 & 0  &  \aug & 0& 1\\
1 & 0  &  \aug & 0& 0\\
0 & 1  &  \aug & 0& 0\\
\end{pmatrix}
+ 0.4 \cdot 
\begin{pmatrix}
0 & 0  &  \aug & 0& 1\\
0 & 0  &  \aug & 1& 0\\
1 & 0  &  \aug & 0& 0\\
0 & 1  &  \aug & 0& 0\\
\end{pmatrix}
\end{align*} 
Note that the way we constructed a doubly stochastic matrix from $A$ is not unique. For any index pair $(i,j), (i',j')$ with $j,j'> k$ we can subtract some value $\beta$ from $a'_{i,j}$ and $a'_{i',j'}$, while adding the same value to $a'_{i',j}$ and $a'_{i,j'}$. The resulting matrix is still a doubly stochastic matrix that fulfills the requirements of the Lemma. In our example we could for example with such operations change $A'$ to 
\[ \begin{pmatrix}
0.2 & 0  &  \aug & 0.8& 0\\
0 & 0.2  &  \aug & 0& 0.8\\
0.8 & 0  &  \aug & 0.2& 0\\
0 & 0.8  &  \aug & 0& 0.2\\
\end{pmatrix} \]
and use this matrix as input for the BvN decomposition. We do not want to be bottlenecked by the remaining values in the extension. In each iteration we can rearrange the values in each row extension such that the full remaining value is lying on one column value. With this realization in mind we propose to instead of extending the rows to full doubly stochastic matrices we suggest using only one value as the remainder for the extension of each row. In our example this would be 
\[ \begin{pmatrix}
0.2 & 0  &  \aug & 0.8\\
0 & 0.2  &  \aug & 0.8\\
0.8 & 0  &  \aug & 0.2\\
0 & 0.8  &  \aug & 0.2\\
\end{pmatrix} \]
In our decomposition we want to split of matrices that are permutation matrices in the first $k$ colums and have the vector $\{\mathds{1}_{\sum_{j<k}a_{i,j}=0}\}_i$ in the extension column.  

Note that we need to consider the remainder value as can be seen in the following example: 
\begin{equation*}
A = 
\begin{pmatrix}
1/3 & 1/3 \\
1/3 & 1/3 \\
1/3  & 1/3 \\
\end{pmatrix}
= 
\begin{pmatrix}
0 & 1 \\
1 & 0 \\
0  & 0 \\
\end{pmatrix}
+
\begin{pmatrix}
1 & 0 \\
0 & 1 \\
0  & 0 \\
\end{pmatrix}
+
\begin{pmatrix}
0 & 0 \\
0 & 0  \\
1/3  & 1/3 \\
\end{pmatrix}
\end{equation*}
After two iterations we are left with a matrix that can not be decomposed into the sum of permutation matrices anymore.
